# Supplementary material for: Rapid Artefact Removal and H&E-Stained Tissue Segmentation
Source: arXiv:2308.13304 source file (2023-12-19)
Supplement: Supplementary file 1 [file supplementry_material_revisions_2.pdf]

# 1 Tissue Masks

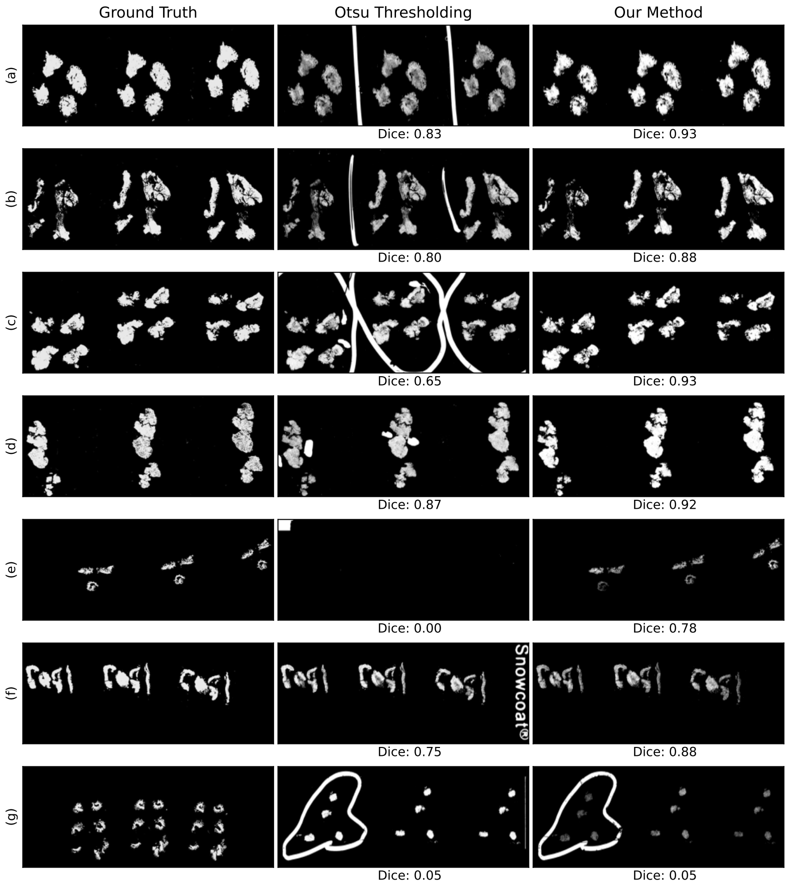


**Suppl. Fig. 1:** Tissue masks and segmentations of WSIs of H&E-stained biopsies containing artefacts of a wide range of types and colours. Left: A manual segmentation of the tissue, considered a ground truth. Middle: The tissue segmentation mask provided by applying Otsu thresholding to the luminance of the WSIs. Right: The tissue segmentation mask provided by our method. The Sørensen-Dice coefficient's between the segmentation and the ground truth are printed below the segmentations. The Sørensen-Dice coefficients in our segmentations are greater than those in Otsu thresholding. We do not expect the Sørensen–Dice coefficients for our segmentations to be 1 as manual tissue segmentation is subjective, containing small pieces of background and missing small pieces of tissue due to human error.

# 2 RGB Cubes

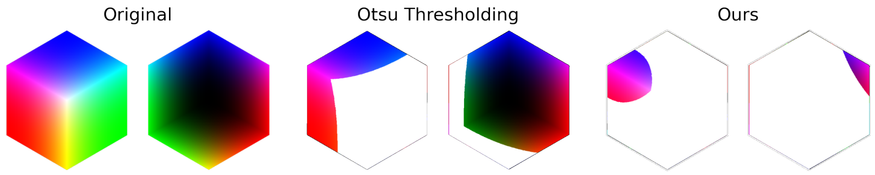


**Suppl. Fig. 2:** The effect of applying Otsu thresholding and our method on a standard 24-bit colour cube. Left: Two 24-bit colour cubes, one with the white corner at the origin and one with the black corner at the origin. Middle: The effect of applying Otsu thresholding on the colour cubes. The darker colours are segmented, and the lighter colours are removed. Right: The effect of applying our method on the colour cubes. The only colours segmented are shades of pink and purple which are the colours that define H&E-stained biopsy tissue.
